# Supplementary material for: Transformers as Support Vector Machines
Source: arXiv:2308.16898 source file (2024-02-22)
Supplement: Supplementary file 1 [file QK_max_margin.tex]

\subsection{Convergence of Gradient Descent  for (K,Q)-Parameterization}\label{sec:KQ convergence proof}

In the following, our objective is to establish analogous assurances for Algorithm \ref{GD-QK} when applied to \eqref{eqn:erm:kq}. Nevertheless, unlike Theorem~\ref{diverg:norm:w}, where a fixed step size of $O(1/L_{\W})$ is utilized, we now necessitate an adaptive step size configuration for the $(\Kb, \Qb)$ decomposition.  This is because $(1/L_\Kb, 1/L_\Qb)$ tends to  $0$ as the number of iterations approaches infinity. To proceed, for any $R > 0$, we introduce the set $\mc{S}(R)$ as follows:
\begin{equation}\label{eqn:kq:set}
 \mc{S}(R):= \left\{(\Kb,\Qb)~~\big|~~\tf{\Qb} \leq R,~~\tf{\Kb} \leq R \right\}.   
\end{equation}
The following lemma demonstrates that given any $R>0$, the number of iterations taken by Algorithm~\ref{GD-QK} within $\Sc(R)$ is finite. 
\begin{lemma}\label{lem:out:S}
Suppose Assumptions~\ref{assum:loss:prope} and \ref{assum:token} hold. Assume the gradient at the initialization $(\Kb(0), \Qb(0))$ is nonzero and $\Lc(\Kb(0), \Qb(0)) \leq \Lc(0, 0)$. Consider Algorithm~\ref{GD-QK} with a step size $\eta=1/L(R)$, where $L(R):=RL_{\W}$. Then for any $R>0$, there exists an iteration index $k$ at which $(\Kb(k),\Qb(k)) \notin \mc{S} (R)$.
\end{lemma}
\begin{proof}
Let us select a value for $R$ and fix the step size to $\eta=1/L(R)$. Assuming that both $(\Kb({k+1}), \Qb(k+1))$ and $(\Kb({k}), \Qb(k))$ reside within the set $\mc{S}(R)$, we can establish a descent of objective analogous to Lemma \ref{lem:grad:descent}. Specifically, we obtain the following result: 
\begin{align}\label{eq:descent:obj}
\nonumber
\mathcal{L}(\Kb({k+1}), \Qb({k+1}))-\mathcal{L}(\Kb({k}),\Qb(k)) &\leq-\frac{1}{2 L(R)} \tf{\nabla \mathcal{L}(\Kb({k}), \Qb(k))}^2 \\
& =-\frac{\eta}{2} \tf{\nabla \mathcal{L}(\Kb({k}), \Qb(k))}^2.
\end{align}
By our assumption, $\tf{\nabla \Lc (\Kb(0), \Qb(0))} \neq 0$, which implies that  %for all $k \geq 1$, 
\begin{equation}\label{eqn:obj:less0}
    \mathcal{L}(\Kb({1}),\Qb(1)) \leq  \mathcal{L}(\Kb({0}),\Qb(0)) - \frac{1}{ 2 L(R)} \tf{\nabla \mathcal{L}(\Kb({0}), \Qb(0))}^2 <    \mathcal{L}(\Kb(0),\Qb(0)) \leq  \mathcal{L}(0,0).
\end{equation}
Next, we claim that for any $R>0$, there exists a constant $\epsilon(R)>0$, such that 
\begin{align}\label{eqn:grad:low:eps}
\forall k\ge1\,:\,  \quad (\Kb (k),\Qb(k)) \in \mathcal{S}, \qquad \tf{\nabla_{\Qb} \Lc(\Kb(k),\Qb(k))}\geq \epsilon(R). 
\end{align}
Fix an arbitrary $R>0$. If \eqref{eqn:grad:low:eps} is not true, then for any $\epsilon>0$, there exists some $k\ge1$ such that $\|\Kb(k)\|_F\le R$ and  $\tf{\Qb(k)} \leq R$ while  \eqref{grad def KQ} gives
\begin{align}\label{eqn:qgrad}
\nonumber
\left\|\nabla_{\Qb} \Lc(\Kb (k),\Qb(k))\right\|_F^2 & =\left\|\frac{1}{n}\sum_{i=1}^n \ell' \left(\bgam_i^\top \sft{\g_i}\right) \cdot \X_i^\top  \sfp{\g_i}  \bgam_i  \z_{i}^\top \Kb(k)\right\|_F^2 \\
&=  \tf{\nabla \Lc (\W(k))}^2 \left\|\Kb(k)\right\|^2_F \leq \epsilon^2,   
\end{align}
where $\g_{i}=\X_i\Kb(k) \Qb(k)^\top\z_{i}=\X_i\W(k)\z_{i}$.

It follows from Lemma~\ref{global des lem} that $\li\nabla\Lc(\W (k)),\Wm/\|\Wm\|_F\ri \leq  - c <0$ for some positive constants $c$.  %\ct{should this be $\langle{\nabla \Lc (\W (k))},{-\Wm/\|\Wm\|_F}\rangle \geq Mc$} 
%Let $-M= \max_{x} \ell'(x)$. Since $\ell'$ is continuous and the domain is bounded, the maximum is attained and negative. 
Hence, $\tf{\nabla \Lc (\W(k))}  \geq c$ and $\tf{\Kb(k)} \leq \epsilon/c$.  This together with $\tf{\Qb(k)} \leq R$ implies that   $\tf{ \Kb(k) \Qb(k)^\top} \leq  \epsilon R/ c$.  In other words,  after $k=1$, $\tf{ \Kb(k) \Qb(k)^\top}$  may be arbitrarily small, which implies $\Lc(\Kb(k), \Qb(k))$ can be arbitrarily close to $ \mathcal{L}(\Kb(0),\Qb(0))$. % \ct{Does this need $K(0)=Q(0)=0$}.
This is a contradiction to \eqref{eqn:obj:less0}. Hence, \eqref{eqn:grad:low:eps} holds.

Now,  it follows from \eqref{eq:descent:obj} and \eqref{eqn:grad:low:eps}  that 
\begin{align*}
  \mathcal{L}(\Kb(0),\Qb(0))
         \ge   \mathcal{L}(\Kb(0),\Qb(0)) -\mathcal{L}_{\star} \geq  \frac{1}{2 L(R)}\sum_{k=0}^{\infty} \left\|\nabla_{\Qb} \Lc(\Kb(k),\Qb(k)) \right\|_{F}^2
         %& =\sum_{t=0}^{\infty}\|W_L\cdots W_2\|^2\|\nR(\wnn)\|^2\dif t \\
        % & %\ge\sum_{t=0}^{\infty}\tf{\Kb(k)}^2~~\tf{\nabla \mc{L}(\W)}^2\\
          \geq \infty,
    \end{align*}
which is a contradiction. Hence,  $(\Kb(k),\Qb(k))$ must go out of $\mc{S} (R)$.
\end{proof}

Note that in Lemma~\ref{lem:out:S},  we assume that the gradients at the initialization $(\Kb(0), \Qb(0))$ are nonzero. Requiring the initialization not to be a critical point is reasonable because if it were, gradient descent would be unable to make any progress.  From Lemma~\ref{lem:out:S}, we see that $(\Kb(k),\Qb(k))$ can go out of the set $\mc{S} (R)$.  However, we can address this matter by dynamically increasing $R$ while proportionally decreasing the step sizes, as formalized in the following theorem:
\begin{theorem}\label{diverg:norm:qk}%\redp{TO FIX}
Suppose Assumption~\ref{assum:loss:prope} on the loss function $\ell$ and Assumption \ref{assum:token} on the tokens hold. Assume the initialization $(\Kb(0), \Qb(0))$ satisfies $\nabla \Lc (\Kb(0),\Qb(0)) \neq 0$. Let $\eta_k=\min\{1/L(R_k),1\}$, where $R_k$ is chosen such that $(\Kb(k),\Qb(k))\in \mc{S}(R_k-1)$, and if $(\Kb(k+1),\Qb(k+1))\in \mc{S} (R_k-1)$, then $R_{k+1}=R_k$.  Then, the following statements hold:
\begin{itemize}
\item %\textbf{No stationary points:} 
There is no $\Kb,\Qb\in\R^{d\times m}$ satisfying $\nabla \Lc(\Kb,\Qb)=0$.
\item Algorithm~\ref{GD-QK} with the step size $\eta_k$  satisfies  $\lim_{k \rightarrow \infty} \tf{\nabla \Lc_\Kb(\Kb(k), \Qb(k))}\vee\tf{\nabla\Lc_\Qb(\Kb(k),\Qb(k))}=0$, and  $\lim_{k\rightarrow\infty} \tf{\Kb(k)}\wedge\tf{\Qb(k)}=\infty$.
\end{itemize}
\end{theorem}

\begin{proof}
Since $(\Kb(k),\Qb(k))\in \mc{S}(R_k)$, %\ct{$S(R_{k}-1)$? But I didn't understand why in Thm. 10 you need $R_{K}-1$}
we have 
    \begin{align}
        \|\Qb(k+1)\|_F \le\|\Qb(k)\|_F+\eta_k\tf{ \nabla_{\Qb} \Lc(\Kb(k),\Qb(k))} \nonumber    & \le\|\Qb(k)\|_F+\frac{1}{L(R_k)}\tf{\nabla_{\Qb} \Lc(\Kb(k),\Qb(k))} \nonumber \\
%         & \le\|\Qb(k)\|_F+\frac{1}{L(R_k)}R_kG \nonumber \\
         & \le\|\Qb(k)\|_F+1. \label{eq:gd_inc}
    \end{align}
%Here the last inequality follows since 
    
Since $R_k\to\infty$ by Lemma~\ref{lem:out:S} and $R_{k+1}=R_k$ as long as $ (\Kb(k+1),\Qb(k+1))\in \mc{S}(R_k-1)$, we obtain
\begin{equation}\label{eqn:c1}
 \max\{ \|\Qb(k)\|_F,  \|\Kb(k)\|_F \} \quad    \textnormal{is unbounded}. \tag{C1}
\end{equation}

It then follows that for any $k$, by Cauchy-Schwarz,
\begin{align*}
\left(\sum_{\tau=0}^{k-1}\eta_{\tau}\right) \left(\sum_{\tau=0}^{k-1}\eta_{\tau} \|\nabla \Lc(\Kb(\tau),\Qb(\tau))\|^2_F\right) & 
\ge \left(\sum_{\tau=0}^{k-1}\eta_{\tau} \|\nabla \Lc(\Kb(\tau),\Qb(\tau))\|^2_F\right)^2\to\infty.
\end{align*}
Since by  \eqref{eq:descent:obj},
\begin{align*}
        \sum_{\tau=0}^{k-1}\eta_{\tau} \left\|\nabla \Lc(\Kb(\tau),\Qb(\tau))\right\|^2_F\le 2\Lc(\Kb(0),\Qb(0))-2\Lc(\Kb(k),\Qb(k) )\le2 \Lc(\Kb(0),\Qb(0)),
\end{align*}
we have $\sum_{t=0}^{\infty}\eta_k=\infty$.

Since gradient descent never increases the risk,  for $(\Kb(k),\Qb(k))\in \mc{S}(R)$, $\|\partial\Lc/\partial \Qb(k)\|_F\ge\epsilon(R)$ for some constant $\epsilon(R)>0$.  Following similar steps  as the proof of \eqref{eqn:grad:low:eps},   we get that $\sum_{k:(\Kb(k),\Qb(k))\in \mc{S}(R)}^{}\eta_k<\infty$.

For simplicity, we  replace $\Qb^\top$ with $\Qb$ in \eqref{eqn:erm:kq}. %Then, for any $(\Kb,\Qb)$, we have 
%     \begin{equation}\label{eq:gd_align_tmp1}
%        \Qb \nabla_{\Qb} \Lc(\Kb,\Qb)^\top= \nabla_{\Kb} \Lc(\Kb,\Qb)   \Kb^{\top} .
%     \end{equation}
 For gradient descent iterates \ref{GD-QK}, summing from $0$ to $k-1$, we get
\begin{align}\label{eqn:qk:recur}
& \quad\Qb(k)^\top\Qb(k)-\Qb(0)^\top\Qb(0)+\sum_{\tau=0}^{k-1}\eta_{\tau}^2 \nabla_{\Qb} \Lc(\Kb(\tau),\Qb(\tau))^\top \nabla_{\Qb} \Lc(\Kb(\tau),\Qb(\tau)) \nonumber \\
= & \quad \Kb(k)\Kb^{\top}(k)-\Kb(0)\Kb^{\top}(0)+\sum_{\tau=0}^{k-1}\eta_{\tau}^2  \nabla_{\Kb} \Lc(\Kb(\tau),\Qb(\tau)) \nabla_{\Kb} \Lc(\Kb(\tau),\Qb(\tau))^\top.
\end{align}
Let
\begin{subequations}
    \begin{align*}
       P_{\Qb}&=\sum_{\tau=0}^{k-1}\eta_{\tau}^2 \nabla_{\Qb} \Lc(\Kb,\Qb) \nabla_{\Qb} \Lc(\Kb(\tau), \Qb (\tau)))^\top,\\
   P_{\Kb}&:=\sum_{\tau=0}^{k-1}\eta_{\tau}^2 \nabla_{\Kb} \Lc(\Kb,\Qb)  \nabla_{\Qb} \Lc(\Kb(\tau), \Kb (\tau)))^\top,
    \end{align*}
    and
\begin{align*}
S_{\Qb}(k)=\sum_{\tau=0}^{k-1}\eta_{\tau}^2 \nabla_{\Qb} \Lc(\Kb(\tau), \Qb (\tau)))^\top \nabla_{\Qb} \Lc(\Kb(\tau), \Qb (\tau))),\\
S_{\Kb}(k)=\sum_{\tau=0}^{k-1}\eta_{\tau}^2 \nabla_{\Kb} \Lc(\Kb(\tau), \Qb (\tau)))^\top \nabla_{\Kb} \Lc(\Kb(\tau), \Qb (\tau))) .
    \end{align*}
\end{subequations}
We obtain
\begin{subequations}
    \begin{align}\label{eq:qk:tr:b1}
           \tr(P_{\Kb}(k))+ \tr(P_{\Qb}(k))  & =\sum_{\tau=0}^{k-1}\eta_{\tau}^2 \|\nabla \Lc(\Kb(\tau), \Qb (\tau))\|^2_F \nonumber \\
         & \le \sum_{\tau=0}^{k-1}\eta_{\tau} \|\nabla \Lc(\Kb(\tau), \Qb (\tau))\|^2_F  \nonumber \\
         &  \leq 2 \Lc(\W(0)) -2 \Lc(\W(k))  \nonumber\\
            &  \leq 2 \Lc(\W(0)) -2 \Lc_\star.
    \end{align}
It follows from \eqref{eqn:qk:recur} that
\begin{align}\label{eq:qk:tr:b2}
\|\Kb(k)\|_F^2=\|\Qb(k)\|_F^2+\|\Kb(0)\|_F^2-\|\Qb(0)\|_F^2-\tr(P_{\Kb}(k))+\tr(S_{\Qb}(k)).
\end{align}    
\end{subequations}
In other words, the difference between the squares of Frobenius norms of $(\Kb,\Qb)$ is still bounded.
% It shows that gradient descent spends a finite amount of time in $\mc{S}$ for any $R>0$.

Now, combining \eqref{eq:qk:tr:b1} and \eqref{eq:qk:tr:b2}, we get
 \begin{align*}
   2 \Lc(\W(0))
           \ge\sum_{t=0}^{\infty} \eta_k \left\|\nabla_{\Qb} \Lc(\Kb (k),\Qb(k))\right\|_F^2 %\\
          %& =\sum_{t=0}^{\infty}\|W_L\cdots W_2\|^2\|\nR(\wnn)\|^2\dif t \\
          %& \ge\sum_{t=0}^{\infty}\|\Kb(k)\|~~\|\nabla \mc{L}(\W) \|\\
           \geq \infty,
     \end{align*}
     which is a contradiction. This implies $\tf{\Kb(k)}\to\infty$, since $\Lc(\Kb,\Qb)$ has no finite optimum.
\end{proof}

Theorem~\ref{diverg:norm:qk} is the formal version of the $(\Kb,\Qb)$-statement in Theorem \ref{diverg:norm:w}. It provides similar guarantees to the $\W$-statements of Theorem \ref{diverg:norm:w}, namely the absence of finite stationary points and the divergence of the parameter norm to infinity. It is important to mention that the step size can be appropriately determined using methods such as a line search. The line search ensures that the \ref{GD-QK} update is not excessively aggressive, thus allowing the boundary $R$ to be increased as needed.
