# Supplementary material for: Transformers as Support Vector Machines
Source: arXiv:2308.16898 source file (2024-02-22)
Supplement: Supplementary file 2 [file toy_dataset.tex]

\section{Toy Dataset for Globally-Convergent Self-Attention}

In this section, we introduce a toy dataset model for which Assumption \ref{assum:nabla0} holds with $\z_i\gets\x_{i1}$. Importantly, this dataset captures the spirit of self-attention by allowing the model to retrieve different output tokens depending on the value of the first token. More concretely, in our model, whenever $\x_1$ admits a value $\ab_j$ from a dictionary $\Ac=\{\ab_j\}_{j=1}^r$, self-attention should retrieve a relevant token $\x_t=\bb_j$ from a dictionary $\Bc=\{\bb_j\}_{j=1}^r$.

%All tokens are centered i.e.~$\E[\x_t]=0$ for all $t\in[T]$. 
\begin{definition} [Toy Distribution for Self-Attn]\label{def data model} Data $(\X,Y)$ is generated according to $\Dc_{\texttt{data}}$ as follows: Let $\rho >1$ be the index of $\x_1$'s \emph{relevant token} (that is allowed to be random).
\begin{itemize}%$\R^d\times \R^d$ with 
\item \textbf{Relevant token:} $(\x_1,\x_\rho)$ has a uniform distribution over $r$ values $(\ab_j,\bb_j)_{j=1}^r$ with associated labels $(y_j)_{j=1}^r$. That is, whenever $(\x_1,\x_\rho)=(\ab_j,\bb_j)$, the output label is $Y=y_j$. 
\item \textbf{Fixed score:} For some $\gamma_1,\gamma_\rho$ and all $j\in[r]$: $y_j \vb^\top\ab_j=\gamma_1$, $y_j \vb^\top\bb_j=\gamma_\rho>0$.
\item \textbf{Other tokens} $t\not\in\{\rho,1\}$ are bounded, independent of the rest, and $\E[\x_t]=\E[\x_t\x_t^\top]\vb=0$.%$\bSi=\E[\x_t\x_t^\top]$ obeys $\bSi\vb=0$.
\end{itemize}
\end{definition}

\redp{Orthogonality condition for concrete example: Suppose vectors $(\ab_j,\bb_j)_{j=1}^r$ are all pairwise orthonormal and other tokens have small projections to the subspace $\text{span}(\ab_j,\bb_j)_{j=1}^r$. First, this would provide a simple explicit example to instantiate Theorem \ref{toy data thm} and Assumption \ref{assume sep}. Second, based on Def.~\ref{def data model}, this would also allow us to discuss the setting where 
\begin{itemize}
\item Self-attention selects $\x_\rho$ if $\gamma_\rho>\gamma_1$.
\item Self-attention selects $\x_1$ if $\gamma_1>\gamma_\rho$.
\end{itemize}
$\gamma_\rho$ vs $\gamma_1$ is related to the following concern: How can our model highlight ``self'' of self-attention?}

\begin{assumption}[Separation] \label{assume sep}Consider the dataset $\Dc_{\texttt{data}}$ of Def.~\ref{def data model}. Let $\W_\rho=\frac{1}{r}\sum_{j=1}^r\bb_j\ab_j^\top$. Assume $|\gamma_1|$ is sufficiently small, $T$ is sufficiently large and for an arbitrarily small $\eps>0$: 
%Scores obey Attention similarities obey 
\begin{align}
\gamma_\rho-y_j\vb^\top \x_t\geq\eps\quad\text{and}\quad (\bb_j-\x_t)^\top\W_\rho\ab_j\geq \eps\quad\text{for all}~j\in[r],t\neq\rho\quad\text{almost surely}.\label{sep condition}
\end{align}
\end{assumption}

\begin{theorem}\label{toy data thm} Consider the dataset model $\Dc_{\texttt{data}}$ of Def.~\ref{def data model}. Denote the initial population gradient $\nabla\Lc(0):=\E_{\Dc_{\texttt{data}}}[\nabla\Lc(0)]$. Let $\W_1=\frac{1}{r}\sum_{j=1}^r\ab_j\ab_j^\top$ and $\W_\rho=\frac{1}{r}\sum_{j=1}^r\bb_j\ab_j^\top$. We have that%For $\X\sim\Dc_{\texttt{data}}$, w
\begin{align}
&\nabla\Lc(0)=\frac{\ell'(0)}{T}(\gamma_1\W_1+\gamma_\rho\W_\rho)-\frac{\ell'(0)}{T^2}(\gamma_1+\gamma_\rho)(\W_1+\W_\rho)\label{eq nablaL0}
\end{align}
Additionally, suppose Assumption \ref{assume sep} holds. Then, $\x_\rho$ is the optimal token and Assumption \ref{assum:nabla0} holds almost surely i.e.
%self-attention at $\nabla\Lc(0)$selects $\x_\rho$
\[
\underset{t\in[T]}{\min}\li(\x_t-\x_\rho)^\top\nabla\Lc(0)\x_1\ri>0.
\]
\end{theorem}
\begin{proof} We will make use of the simple structure of softmax at $\W=0$. Let $\bgam=Y\cdot\X\vb$ and $\Fb_t=\x_t\x_1^\top$. Using the fact that softmax derivative at $0$ is simply all $1/T$ vector, we have that
\begin{align}
\nabla\Lc(0)=\frac{\ell'(0)}{T}\E[\sum_{t=1}^T \bgam_t\Fb_t]-\frac{\ell'(0)}{T^2}\E[\sum_{t=1}^T \bgam_t\sum_{t=1}^T \Fb_t].
\end{align}
%y_j\vb^\top\ab_j%\vb^\top\bb_j
Let $\bSi=\E[\x_t\x_t^\top]$ for $t\notin\{1,\rho\}$. To proceed, observe that, for $t\not\in\{1,\rho\}$
\[
\E[\bgam_t\Fb_t]=\E[Y\vb^\top\x_t\x_t\x_1^\top]=\E[\vb^\top\x_t\x_t]\E[Y\x_1]^\top=\bSi\vb\E[Y\x_1]^\top=0.
\]
Similarly for $t\not\in\{1,\rho\}$, we have $\E[\sum_{i=1}^T \bgam_i\Fb_t]=0$ by additionally using $\E[\x_t]=0$.

What remains is $t=1$ and $t=\rho$. Using fixed score assumption, we find
\[
\E[\bgam_1\Fb_1]=\E[Y\vb^\top\x_1\x_1\x_1^\top]=\gamma_1\W_1,\quad\E[\bgam_\rho\Fb_\rho]=\E[Y\vb^\top\x_\rho\x_\rho\x_1^\top]=\gamma_\rho\W_\rho.
\]
Similarly, we obtain
\[
\E[\sum_{t=1}^T \bgam_t\sum_{t=1}^T \Fb_t]=\frac{1}{T^2}(\gamma_1+\gamma_\rho)(\W_1+\W_\rho),
\]
to conclude with \eqref{eq nablaL0}. To conclude with Assumption \ref{assum:nabla0}, we use Assumption \ref{assume sep} and observe that $T\nabla\Lc(0)$ is arbitrarily close to $T\hat{\nabla}\Lc(0)$ where $\hat{\nabla}\Lc(0)=\frac{\ell'(0)\gamma_\rho}{T}\W_\rho$. Now, recalling $\ell'(0)<0$, applying the right hand-side of \eqref{sep condition} with $\hat{\nabla}\Lc(0)\propto-\W_\rho$, and using the boundedness of tokens and $\eps>0$ as perturbation buffer, we obtain the desired statement.
\end{proof}
